# Supplementary material for: Multiwavelength Modeling for the Shallow Decay Phase of Gamma-Ray Burst Afterglows
Source: arXiv:2404.09675 source file (2024-07-22)
Supplement: Supplementary file 1 [file APPENDIX.tex]

%\section{Gamma-ray Background (MAYBE NOT NECESSARY)}
%The isotropic component of the extragalactic gamma-ray background (EGB) is measured by the Fermi observation \citep[][]{Ackermann2015}.
%In this section, we check that the gamma-ray background in our model does not overproduce the upper limit for the nonblazar component of the EGB intensity \citep[][]{Ackermann_PhysRevLett.116.151105}}.
%The mass luminosity relation for the gamma-ray is derived under the same assumption as Section~\ref{subsec:L_evolution}.
